# Supplementary material for: Perovskite-type cobalt oxide at the multiferroic Co/Pb Zr$_{0.2}$Ti$_{0.8}$O$_{3}$ interface
Source: arXiv:2004.00489 source file (2020-04-01)
Supplement: Supplementary file 1 [file SupportingInformation.pdf]

# Supporting Information
for *Adv. Mater.,*

# Perovskite-type cobalt oxide at the multiferroic Co/Pb $Zr_{0.2}Ti_{0.8}O_3$ interface

*K. Mohseni, A. Polyakov, H. B. Vasili, I. V. Maznichenko, S. Ostanin, A.Quindeau, N. Jedrecy, E. Fonda, L. V. Bekenov, V. N. Antonov, P. Gargani, M. Valvidares, I. Mertig, S. S. P. Parkin, A. Ernst, and H. L. Meyerheim*

## I. SXRD structure analysis for 0.5 ML Co/PZT/LSMO/STO(001)

Apart from the experiment discussed in the main text, additional data were collected on another PZT/LSMO/STO(001) sample on which approximately 0.5 ML of cobalt was deposited in-situ. The X-ray diffraction experiment was subsequently carried out in the same way as done for the 1 ML sample discussed in the main text. Symbols in Figure S1 represent the experimental structure factor magnitudes [$|F_{obs}$ (HKL)|] along six symmetry independent crystal truncation rods (CTRs) together with their standard uncertainties represented as error bars. Solid lines represent the best fit of the calculated structure factor magnitudes [$|F_{calc}$ (HKL)|] to the observed ones, which is quantified by the un-weighted residual (Ru) and the Goodness of fit (GOF) parameter [1] being 0.17 and 1.51, respectively.

Direct eye inspection reveals that the $|F_{cal}$ (HKL)| fit the $|F_{obs}$ (HKL)| almost perfectly except in the regime near the bulk Bragg-reflections as well as in the low $q_z$ region along the (10L) rod, very similar to case of the 1 ML sample (see Figure 1) in the main text. The latter is attributed to spurious intensity originating from the sample *not* related to the Co/PZT/LSMO structure. Also, intensity integration at low $q_z$ and close to bulk Bragg reflections may fundamental difficulties as discussed in Ref. [1].

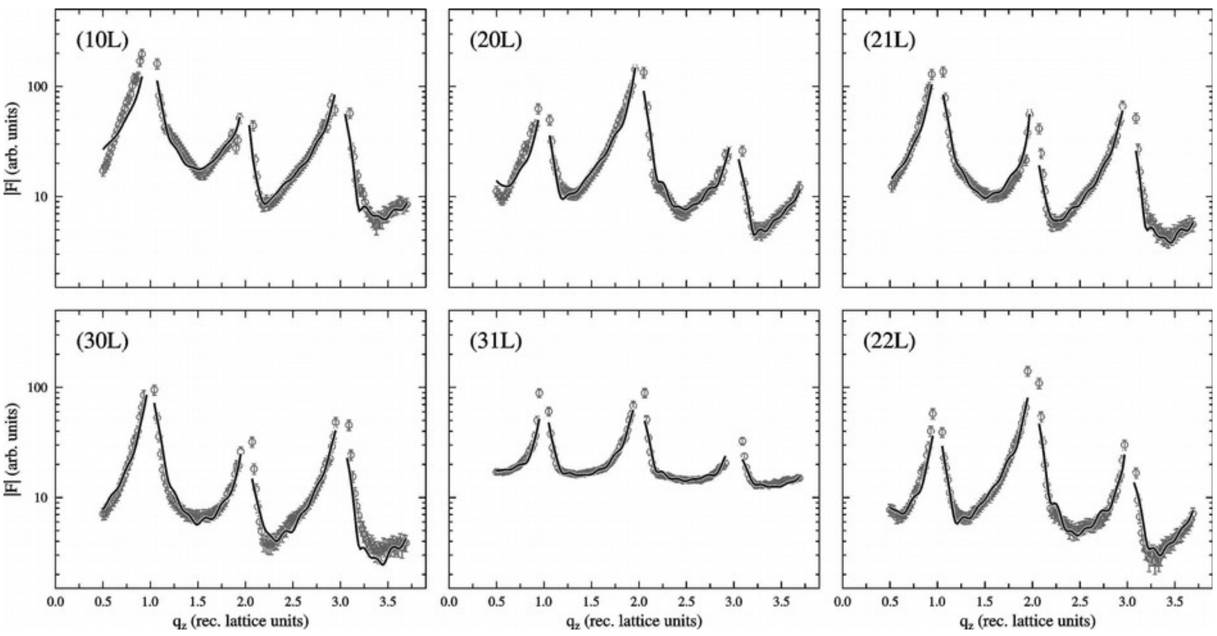


*Figure S1: Experimental (symbols) and fitted (lines) structure factor magnitudes [|F(HKL)|] for 0.5 Ml Co/PZT/LSM/STO(001) along six symmetry independent crystal truncation rods. Error bars represent 1σ uncertainties derived from the quadrature sum of the statistical uncertainty and the reproducibility of symmetry equivalent reflections.*

The fit to the $F_{obs}$(HKL) was performed in the same way as for the 1 ML sample discussed in the main text, based on the p4mm plane group symmetry.

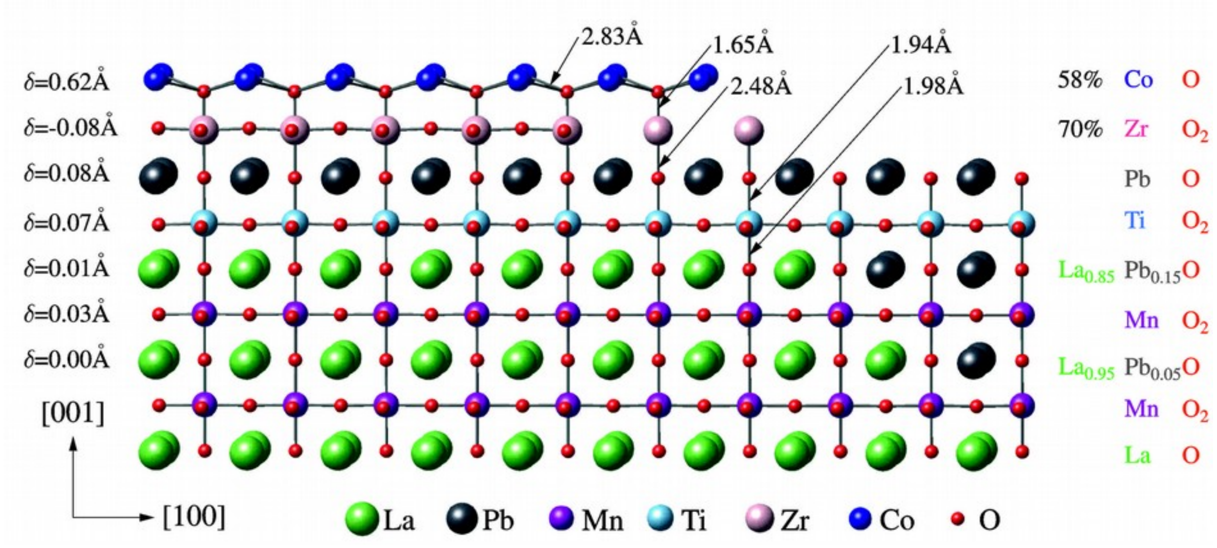

*Figure S2: Schematic of the near surface structure of 0.5 ML Co/PZT/LSMO/STO(001) as derived from the CTR data shown in Figure S1. Differently colored balls represent atomic species as given in the legend. The approximate stoichiometry within each layer is given on the right. Some interatomic distances and the parameter δ (intralayer-spacings between the cations and oxygen atom) are listed in ÅngstrØm units.*

The most important result is that deposited cobalt is oxidized to form a fractionally (≈50-60%) filled CoO layer on the $Ti(Zr)O_2$ termination layer of the PZT layer. In this respect, this sample represents an earlier stage of the oxide interface formation prior to the growth of the second $CoO_2$ layer, which is observed after deposition of 1 ML cobalt. From the amount of cobalt deposited (≈0.50 ML) and the fractional coverage we may conclude that all deposited cobalt is oxidized and no (disordered) cobalt metal is present on the surface which may escape determination by SXRD.

At a closer look into the structure it is noteworthy that the CoO-layer has a high positive δ-value (0.62 Å), in analogy to δ=0.49 Å found for the CoO-layer in the 1 ML sample (see Figure 3 of the main text), while all other δ-values are relatively low (0.08 Å at most). The shortest metal-oxygen distance (1.65 Å) is the one along the vertical between oxygen in the CoO layer and the zirconium atom in terminating $ZrO_2$ layer of the PZT film: The same value is also observed for the 1 ML sample (see Figure 3 in the main text). We attribute this very short distance to two reasons: (i) reduced coordination number of the surface layer oxygen atoms and (ii) the presence of large (static) disorder in the CoO layer. Refinement of the Debye-parameter ($B=8\pi^2\langle u\rangle^2$) [2] for these atoms yields values in the range between 6 to 8 $Å^2$, corresponding to a root mean square displacement amplitude of $\sqrt{\langle u\rangle^2}=0.3$ Å. This considerably large disorder likely involves a non-Gaussian distribution of the probability density function, which –however- is neglected in the "conventional" analysis based on the

(Gaussian) Debye-Waller type formalism. This simplification is known to lead to artificially reduced interatomic distances by up to typically 0.1 Å. For details, we refer to Refs. [2, 3]. Other parts of the structure including the PZT and the LSMO film closely resemble those of the 1 ML sample. For instance, there is Pb/La cationic exchange in the 20% range, albeit affecting only three layers instead of four. The degree of cationic intermixing might sensitively depend on the film growth parameters during the pulsed laser deposition process, which –however- was no further investigated in this study. Finally, as in the case of the 1ML sample there is some evidence for an enrichment of zirconium at the boundaries of the PZT film, here solely on the top, while at both sides in the case of the 1 ML sample. We tentatively suggest that this surface enrichment of zirconium over titanium as compared to the target stoichiometry $Ti_{0.80}$ $Zr_{0.20}$ might be responsible for the polarization enhancement in PZT in comparison with pure $PbTiO_3$ [4].

## II. EXAFS analysis of 1ML Co/PZT/LSMO/STO(001) annealed in oxygen

In the main text we have discussed the EXAFS analysis of the short range order at the Co/PZT interface after deposition of approximately 1 ML of cobalt. In a subsequent experiment we have annealed this sample at about 450°C under oxygen partial pressure of $p_{O2}$ $=10^{-6}$ mbar in order to form the thermodynamically stable CoO phase which in the bulk crystallizes in the cubic sodium-chloride structure type. Data were monitored in the $E_{||}$ geometry above the Co-K absorption edge ($E_0$=7707 eV) in the fluorescence yield (FY) mode as shown on Figure S3 (a). The $k^2$-weighted interference function [$\chi(k)$] plotted versus k, the magnitude of the photoelectron's wave vector is presented in the inset.

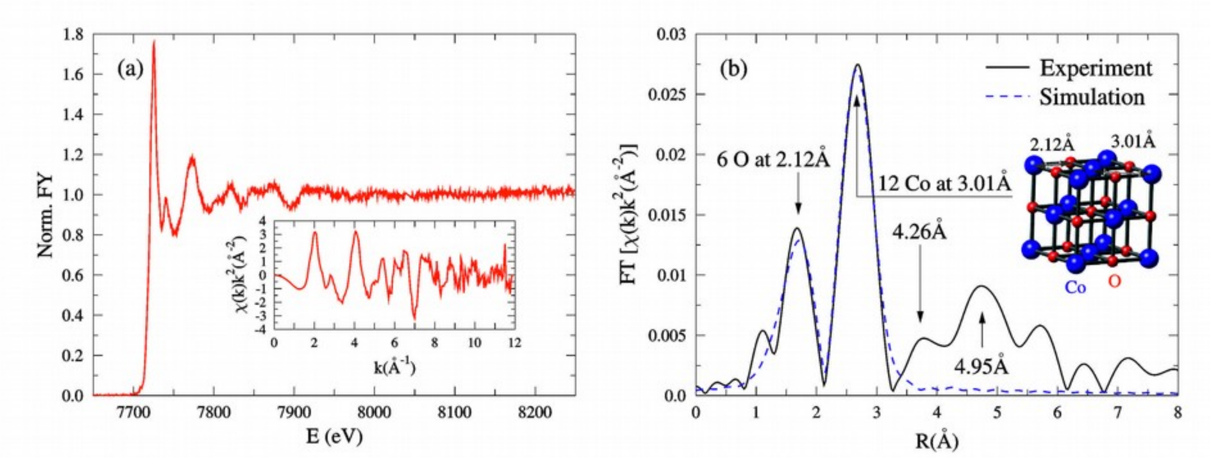


*Figure S3: (a) EXAFS spectrum measured in the $E_{//}$ geometry above the Co-K absorption edge for 1 ML Co on PZT/LSMO after annealing at 450°C under $p_{O2}=10^{-6}$ mbar oxygen atmosphere. The inset shows the $k^2$-weighted interference function [$\chi(k)$] versus k, the wave vector of the photoelectron. (b): Magnitude of the Fourier-Transform (FT) of $\chi(k)\cdot k^2$ (solid line). The dotted line represents a fit to the FT based on the structure model of cubic CoO schematically given on the right (for details see text).*

Comparison with the spectra for the as-deposited sample (see Figure 4 in the main text) gives clear evidence for an enhanced amplitude and the presence of higher order shells. The solid line in Figure S3 (b) is the Fourier-Transform (FT) of $\chi(k)\cdot k^2$ which is plotted together with the fitted FT represented by the dashed line. The analysis is based on R-space fitting using theoretical phases and amplitudes as discussed in the main text. The FT in Figure S3(b) is characterized by several peaks, the most prominent ones being related to the first and second shell in CoO. These correspond to $N_1$*=6 oxygen atoms at $R_1$=2.12 Å and $N_2$*=12 cobalt atoms at $R_2$=3.01 Å in almost perfect agreement with expected values for cubic CoO with lattice parameter 4.26 Å. The smaller peaks beyond the 3 Å regime correspond to higher shells. For instance, both peaks indicated by arrows correspond to neighbors (path lengths) of 4.26 Å and 4.95 Å, respectively. The first related to R=4.26 Å is attributed to neighbor atoms

at a distance of one lattice parameter. Here, the photoelectron experiences multiple scattering by the intervening oxygen atom inducing an enhancement of the scattering amplitude [5].

The second peak, which corresponds to R=4.95 Å is attributable to several multiple scattering paths. We have not included these higher shells into the quantitative fit, as these are not important in the context of our study. In summary, a bulk-like CoO phase forms upon annealing the as deposited Co/PZT interface under oxygen atmosphere. Fixing the effective coordination numbers for $N_1$*=6 and $N_2$*=12 we have obtained the amplitude reduction factor $S^2_0$=0.90, which we have used throughout the analysis of the Co/PZT interface structures.

References:

[1] J. Drnec, T. Zhou, S. Pintea, W. Onderwater, E. Vlieg, G. Renaud, and R. Felici, J. Appl. Cryst. **2014**, 47, 365

[2] W. F. Kuhs, Acta Cryst. **1992**, A 48, 80

[3] H. L. Meyerheim and W. Moritz, Appl. Phys **1998**, A 67, 645.

[4] V.S. Borisov, S. Ostanin, I.V. Maznichenko, A. Ernst, and I. Mertig, Phys. Rev. **2014**, B 89, 054436

[5] D.C. Koningsberger, and R. Prins, "X-Ray Absorption", John Wiley and Sons (New York, 1988)
